# Supplementary material for: SoccerNet-Tracking: Multiple Object Tracking Dataset and Benchmark in Soccer Videos
Source: arXiv:2204.06918 source file (2022-04-20)
Supplement: Supplementary file 1 [file 7_supplementary.tex]

\section{Supplementary Material}
